# Supplementary material for: A Numerical Framework for Efficient Motion Estimation on Evolving Sphere-Like Surfaces based on Brightness and Mass Conservation Laws
Source: arXiv:1805.01006 source file (2018-05-02)
Supplement: Supplementary file 1 [file appendix.tex]

\section{Definitions}

For $t \in I$, let $\Sigma \subseteq \mathcal{M}_{t}$ be connected and let $\partial \Sigma$ denote its boundary.
For $x \in \partial \Sigma$, we denote by $\boldsymbol{\hat{\nu}}(t, x) \in \R^{3}$ the exterior outward unit normal field, which is normal to $\partial \Sigma$ and tangent to $\mathcal{M}_{t}$.

For a tangent vector field $\mathbf{\hat{v}} = v^{i} \partial_{i} \y$, we denote by $(\mathbf{\hat{v}})_{\Sigma} = (v^{i})_{\Sigma} \partial_{i} \y$ the (component-wise) average tangent vector field, where $(v^{i})_{\Sigma} \coloneqq \frac{1}{\abs{\Sigma}} \int_{\Sigma} v^{i} \; d\Sigma$.

For $\Sigma \subseteq \mathcal{M}_{t}$, we define the $H^{1}(\Sigma)$ Sobolev semi-norm as
\begin{equation}
	\abs{\mathbf{\hat{v}}(t, \cdot)}_{H^{1}(\Sigma)}^{2} \coloneqq \int_{\Sigma} \norm{\nabla \mathbf{\hat{v}}(t, \cdot)}_{2}^{2} \; d\Sigma
\label{eq:h1seminorm}
\end{equation}
and the Sobolev space $H^{1}(\Sigma)$ as the completion of $C^{\infty}(\Sigma)$ tangent vector fields with respect to the norm
\begin{equation}
	\norm{\mathbf{\hat{v}}(t, \cdot)}_{H^{1}(\Sigma)}^{2} \coloneqq \norm{\mathbf{\hat{v}}(t, \cdot)}_{L^{2}(\Sigma)}^{2} + \abs{\mathbf{\hat{v}}(t, \cdot)}_{H^{1}(\Sigma)}^{2}.
\label{eq:h1norm}
\end{equation}

\begin{remark} \label{rem:seminorm}
Let us add that, for $\Sigma = \mathcal{M}_{t}$, \eqref{eq:h1seminorm} is actually a norm whenever $\mathcal{M}_{t}$ is diffeomorphic to the 2-sphere since, by virtue of the Hairy Ball Theorem, no covariantly constant tangent vector field but $\mathbf{\hat{v}} = 0$ exists, see e.g.~\cite[p.~125]{Hir94}.
\end{remark}

For a tangent vector field $\mathbf{\hat{v}} = v^{i} \partial_{i} \y$, its surface divergence is defined as
\begin{equation}
	\nabla_{\mathcal{M}} \cdot \mathbf{\hat{v}} = \Tr(\nabla \mathbf{\hat{v}}) = \sum_{i = 1}^{2} \nabla_{\mathbf{\hat{e}}_{i}} \mathbf{\hat{v}} \cdot \mathbf{\hat{e}}_{i} = \mathfrak{D}_{i}\mathfrak{v}^{i},
\label{eq:surfdiv}
\end{equation}
where $\{\mathbf{\hat{e}}_{1}, \mathbf{\hat{e}}_{2}\}$ is an orthonormal basis of the tangent space and $\mathfrak{D}_{i}\mathfrak{v}^{i}$ is defined analogous to \eqref{eq:covderivcoeff}, see \cite{Lee97} for details.
We define the space $H^{\mathrm{div}}(\mathcal{M}_{t} \setminus \Sigma)$ as the completion of $C^{\infty}(\mathcal{M}_{t} \setminus \Sigma)$ tangent vector fields with respect to the norm
\begin{equation*}
	\norm{\mathbf{\hat{v}}(t, \cdot)}_{H^{\mathrm{div}}(\mathcal{M}_{t} \setminus \Sigma)}^{2} \coloneqq \norm{\mathbf{\hat{v}}(t, \cdot)}_{L^{2}(\mathcal{M}_{t} \setminus \Sigma)}^{2} + \norm{\nabla_{\mathcal{M}} \cdot \mathbf{\hat{v}}(t, \cdot)}_{L^{2}(\mathcal{M}_{t} \setminus \Sigma)}^{2}.
\end{equation*}

\section{Wellposedness of Optical Flow}

In what follows we keep $t \in I$ arbitrary but fixed.
For $\Sigma \subseteq \mathcal{M}_{t}$, we define the space $X \coloneqq H^{1}(\Sigma) \times L^{2}(\mathcal{M}_{t} \setminus \Sigma)$ with respect to the norm
\begin{equation}
	\norm{\mathbf{\hat{w}}}_{X}^{2} \coloneqq \norm{\mathbf{\hat{w}}}_{H^{1}(\Sigma)}^{2} + \norm{\mathbf{\hat{w}}}_{L^{2}(\mathcal{M}_{t} \setminus \Sigma)}^{2},
\label{eq:normx}
\end{equation}
see \eqref{eq:h1norm} for the definition of the $H^{1}(\Sigma)$ norm.
For an element $\mathbf{\hat{w}} = (\mathbf{\hat{w}}_{1}, \mathbf{\hat{w}}_{2}) \in X$, the norms are taken with regard to the projections $\mathbf{\hat{w}}_{1} = \mathbf{\hat{w}}|_{\Sigma}$ and $\mathbf{\hat{w}}_{2} = \mathbf{\hat{w}}|_{\mathcal{M}_{t} \setminus \Sigma}$.

In what follows, we seek a minimiser to the energy $\mathcal{E}: X \to [0, +\infty]$,
\begin{equation}
	\mathcal{E}(\mathbf{\hat{w}}) \coloneqq \norm{d_{t}^{\mathbf{\hat{V}}} \hat{f} + \nabla_{\mathcal{M}} \hat{f} \cdot \mathbf{\hat{w}}}_{L^{2}(\mathcal{M}_{t})}^{2} + \mathcal{R}(\mathbf{\hat{w}}),
\label{eq:offunctional}
\end{equation}
where, given a measurable function $s(t, \cdot): \mathcal{M}_{t} \to \{0, 1\}$, the regularisation functional $\mathcal{R}(\mathbf{\hat{w}})$ is defined as
\begin{equation}
	\mathcal{R}(\mathbf{\hat{w}}) \coloneqq \alpha_{0} \int_{\mathcal{M}_{t}} s \norm{\nabla \mathbf{\hat{w}}}_{2}^{2} \; d\mathcal{M}_{t} + \alpha_{1} \int_{\mathcal{M}_{t}} (1-s) \norm{\mathbf{\hat{w}}}^{2} \; d\mathcal{M}_{t},
\label{eq:regfunctional}
\end{equation}
and $\alpha_{0}, \alpha_{1} > 0$ are regularisation parameters.
For simplicity of the analysis we assume that $s$ is the characteristic function of $\Sigma$, ideally a segmentation of the cells.
As a consequence, we can later identify the terms with the norms in \eqref{eq:normx}.
The idea behind $\mathcal{R}(\mathbf{\hat{w}})$ is that it favours vector fields of certain regularity in areas where microscopy data is present but, on the other hand, prevents undesired fill-in effects in regions with no data.

For simplicity of the analysis of the variational properties of $\mathcal{E}$ we assume that $\Sigma \subseteq \mathcal{M}_{t}$ consists of only one connected region.
Moreover, we require the following two lemmata.
The first is analogous to \cite[Chap.~5, Thm.~1]{Eva10}:

\begin{lemma}[Poincaré-Wirtinger inequality] \label{lem:poincarewirtinger}
Let $\Sigma \subset \mathcal{M}_{t}$ be open, connected, and let $\partial \Sigma$ be in $C^{1}$.
Then, there exists some $C > 0$ such that for all $\mathbf{\hat{w}} \in H^{1}(\Sigma)$,
\begin{equation}
	\norm{\mathbf{\hat{w}} - (\mathbf{\hat{w}})_{\Sigma}}_{L^{2}(\Sigma)}^{2} \le C \abs{\mathbf{\hat{w}}}_{H^{1}(\Sigma)}^{2}.
\label{eq:poincareineq}
\end{equation}
\end{lemma}
See Appx.~\ref{sec:deferredproofs} for a proof.
Here, $(\mathbf{\hat{w}})_{\Sigma}$ denotes the component-wise average, cf. Sec.~\ref{sec:background}.
The second lemma is based on \cite[p.~29]{Schn91a}:

\begin{lemma} \label{lem:schnoerrineq}
Let $\Sigma \subseteq \mathcal{M}_{t}$.
Moreover, let $\hat{f}(t, \cdot): \mathcal{M}_{t} \to \R$ and let $\y(t, \cdot): \Omega \to \mathcal{M}_{t}$ be a regular parametrisation such that $\partial_{1} f$ and $\partial_{2} f$ are linear independent, that is
\begin{equation}
	\abs{\langle \partial_{1} f, \partial_{2} f \rangle_{L^{2}(\Sigma)}} < \norm{\partial_{1} f}_{L^{2}(\Sigma)} \norm{\partial_{2} f}_{L^{2}(\Sigma)}.
\label{eq:linindep}
\end{equation}
Then, for $\mathbf{\hat{w}} = w^{i} \partial_{i} \y \in L^{2}(\Sigma)$ with both $w^{1}$ and $w^{2}$ constant, there exists a constant $C > 0$ such that
\begin{equation}
	\norm{\mathbf{\hat{w}}}_{L^{2}(\Sigma)}^{2} \le C \norm{\nabla_{\mathcal{M}} \hat{f} \cdot \mathbf{\hat{w}}}_{L^{2}(\Sigma)}^{2}.
\label{eq:schnoerrineq}
\end{equation}
\end{lemma}
See Appx.~\ref{sec:deferredproofs} for a proof.
In what follows, we let $x \lesssim y$ be short for $x \le C y$ for some constant $C > 0$ and denote by $W^{1, \infty}(\mathcal{M}_{t})$ functions with essentially bounded weak derivative.
We apply the direct method in the calculus of variations \cite{Dac08} and show the following:

\begin{theorem} \label{thm:ofwellposedness}
Let $\hat{f} \in W^{1, \infty}(\mathcal{M}_{t})$ and let $d_{t}^{\mathbf{\hat{V}}} \hat{f} \in L^{2}(\mathcal{M}_{t})$.
Moreover, let $\hat{f}$, $\y$, and $\Sigma$ satisfy the assumptions of Lemmata~\ref{lem:poincarewirtinger} and \ref{lem:schnoerrineq}.
Then, there exists a unique minimiser of $\mathcal{E}$ in the space $X$.
\end{theorem}
\begin{proof}
By Remark~\ref{rem:seminorm}, wellposedness immediately follows if $\Sigma = \mathcal{M}_{t}$, see \cite{BauGraKir15, LefBai08}.
Hence, it suffices to consider $\Sigma \subset \mathcal{M}_{t}$.

First, we show that $\mathcal{E}$ is proper, coercive, and weakly lower-semicontinuous.
We can then apply \cite[Thm.~3.30]{Dac08} to obtain the existence of a minimiser.

From non-negativity of $\mathcal{E}$ and the assumptions on $\hat{f}$ we find that $\mathcal{E}$ is proper.
For coercivity we show that $\norm{\mathbf{\hat{w}}}_{X}^{2} - b \lesssim \mathcal{E}(\mathbf{\hat{w}})$ for all $\mathbf{\hat{w}} \in X$ and some $b \ge 0$:
\begin{align*}
	\norm{\mathbf{\hat{w}}}_{X}^{2} & = \norm{\mathbf{\hat{w}}}_{L^{2}(\Sigma)}^{2} + \abs{\mathbf{\hat{w}}}_{H^{1}(\Sigma)}^{2} + \norm{\mathbf{\hat{w}}}_{L^{2}(\mathcal{M}_{t} \setminus \Sigma)}^{2} \\
	& \lesssim \norm{(\mathbf{\hat{w}})_{\Sigma}}_{L^{2}(\Sigma)}^{2} + \norm{\mathbf{\hat{w}} - (\mathbf{\hat{w}})_{\Sigma}}_{L^{2}(\Sigma)}^{2} + \abs{\mathbf{\hat{w}}}_{H^{1}(\Sigma)}^{2} + \norm{\mathbf{\hat{w}}}_{L^{2}(\mathcal{M}_{t} \setminus \Sigma)}^{2} \\
	& \overset{\mathclap{\eqref{eq:poincareineq}}}{\lesssim} \norm{(\mathbf{\hat{w}})_{\Sigma}}_{L^{2}(\Sigma)}^{2} + \abs{\mathbf{\hat{w}}}_{H^{1}(\Sigma)}^{2} + \norm{\mathbf{\hat{w}}}_{L^{2}(\mathcal{M}_{t} \setminus \Sigma)}^{2} \\
	& \overset{\mathclap{\eqref{eq:schnoerrineq}}}{\lesssim} \norm{\nabla_{\mathcal{M}} \hat{f} \cdot (\mathbf{\hat{w}})_{\Sigma}}_{L^{2}(\Sigma)}^{2} + \abs{\mathbf{\hat{w}}}_{H^{1}(\Sigma)}^{2} + \norm{\mathbf{\hat{w}}}_{L^{2}(\mathcal{M}_{t} \setminus \Sigma)}^{2} \\
	& \lesssim \norm{\nabla_{\mathcal{M}} \hat{f} \cdot \mathbf{\hat{w}}}_{L^{2}(\Sigma)}^{2} + \norm{\nabla_{\mathcal{M}} \hat{f} \cdot (\mathbf{\hat{w}} - (\mathbf{\hat{w}})_{\Sigma})}_{L^{2}(\Sigma)}^{2} + \abs{\mathbf{\hat{w}}}_{H^{1}(\Sigma)}^{2} + \norm{\mathbf{\hat{w}}}_{L^{2}(\mathcal{M}_{t} \setminus \Sigma)}^{2} \\
	& \lesssim \norm{\nabla_{\mathcal{M}} \hat{f} \cdot \mathbf{\hat{w}}}_{L^{2}(\mathcal{M}_{t})}^{2} + \abs{\mathbf{\hat{w}}}_{H^{1}(\Sigma)}^{2} + \norm{\mathbf{\hat{w}}}_{L^{2}(\mathcal{M}_{t} \setminus \Sigma)}^{2} \\
	& \lesssim \mathcal{E}(\mathbf{\hat{w}}) + \norm{d_{t}^{\mathbf{\hat{V}}} \hat{f}}_{L^{2}(\mathcal{M}_{t})}^{2},
\end{align*}
where we have used the parallelogram law, the Cauchy–Schwarz inequality, and $\hat{f} \in W^{1, \infty}(\mathcal{M}_{t})$.

Note that $\mathcal{E} = \mathcal{E}|_{\Sigma} + \mathcal{E}|_{\mathcal{M}_{t} \setminus \Sigma}$ and by the same arguments we find that each of $\mathcal{E}|_{\Sigma}$ and $\mathcal{E}|_{\mathcal{M}_{t} \setminus \Sigma}$ is coercive with regard to $H^{1}(\Sigma)$ and $L^{2}(\mathcal{M}_{t} \setminus \Sigma)$, respectively.
Weak lower-semicontinuity of $\mathcal{E}$ follows immediately by showing that each term in the sum is weakly lower-semicontinuous.

Let $\{ \mathbf{\hat{w}}_{n} \} \subset X$ converge weakly to $\mathbf{\hat{w}}_{0} \in X$.
In particular, since $X$ is a Hilbert space, $\mathbf{\hat{w}}_{n} \rightharpoonup \mathbf{\hat{w}}_{0}$ in $H^{1}(\Sigma)$ and $\mathbf{\hat{w}}_{n} \rightharpoonup \mathbf{\hat{w}}_{0}$ in $L^{2}(\mathcal{M}_{t} \setminus \Sigma)$, where we have omitted the restrictions $|_{\Sigma}$ and $|_{\mathcal{M}_{t} \setminus \Sigma}$, respectively.
Taking into account Kondrakov's Theorem for Riemannian manifolds \cite[Thm.~2.34]{Aub82} and rewriting $\mathcal{E}|_{\Sigma}$ with the help of \eqref{eq:surfintegralcoord} we can apply \cite[Thm.~3.23]{Dac08}, since the integrand is convex in $\nabla \mathbf{\hat{w}}$ and coercive.
Similarly, we apply \cite[Thm.~3.20]{Dac08} to $\mathcal{E}|_{\mathcal{M}_{t} \setminus \Sigma}$ and conclude the existence of a minimiser.

To establish uniqueness we denote by $m \coloneqq \inf_{\mathbf{\hat{w}} \in X} \mathcal{E}(\mathbf{\hat{w}})$.
Let $\mathbf{\hat{u}}, \mathbf{\hat{v}} \in X$ such that $\mathcal{E}(\mathbf{\hat{u}}) = \mathcal{E}(\mathbf{\hat{v}})  = m$.
For $U \subseteq \mathcal{M}_{t}$, the parallelogram law yields
\begin{equation*}
	\lnorm{\frac{u + v}{2}}_{L^{2}(U)}^{2} = \frac{1}{2} \norm{u}_{L^{2}(U)}^{2} + \frac{1}{2} \norm{v}_{L^{2}(U)}^{2} - \lnorm{\frac{u - v}{2}}_{L^{2}(U)}^{2}.
\end{equation*}
We apply it to $u = d_{t}^{\mathbf{\hat{V}}} \hat{f} + \nabla_{\mathcal{M}} \hat{f} \cdot \mathbf{\hat{u}}$ and $v = d_{t}^{\mathbf{\hat{V}}} \hat{f} + \nabla_{\mathcal{M}} \hat{f} \cdot \mathbf{\hat{v}}$ for $U = \mathcal{M}_{t}$.
Then, to $u = \nabla \mathbf{\hat{u}}$ and $v = \nabla \mathbf{\hat{v}}$ for $U = \Sigma$.
And finally, to $u = \mathbf{\hat{u}}$ and $v = \mathbf{\hat{v}}$ for $U = \mathcal{M}_{t} \setminus \Sigma$.
By adding these three identities we obtain
\begin{equation*}
\begin{aligned}
	\mathcal{E} \left( \frac{\mathbf{\hat{u}} + \mathbf{\hat{v}}}{2} \right) = \frac{1}{2} \mathcal{E}(\mathbf{\hat{u}}) + \frac{1}{2} \mathcal{E}(\mathbf{\hat{v}}) & - \frac{1}{4}\norm{\nabla_{\mathcal{M}} \hat{f} \cdot (\mathbf{\hat{u}} - \mathbf{\hat{v}})}_{L^{2}(\mathcal{M}_{t})}^{2} \\
	& - \frac{\alpha_{0}}{4} \abs{\mathbf{\hat{u}} - \mathbf{\hat{v}}}_{H^{1}(\Sigma)}^{2} - \frac{\alpha_{1}}{4} \norm{\mathbf{\hat{u}} - \mathbf{\hat{v}}}_{L^{2}(\mathcal{M}_{t} \setminus \Sigma)}^{2}.
\end{aligned}
\end{equation*}
Then,
\begin{equation*}
\begin{aligned}
	m \le \mathcal{E} \left( \frac{\mathbf{\hat{u}} + \mathbf{\hat{v}}}{2} \right) = m & - \frac{1}{4}\norm{\nabla_{\mathcal{M}} \hat{f} \cdot (\mathbf{\hat{u}} - \mathbf{\hat{v}})}_{L^{2}(\mathcal{M}_{t})}^{2} \\
	& - \frac{\alpha_{0}}{4} \abs{\mathbf{\hat{u}} - \mathbf{\hat{v}}}_{H^{1}(\Sigma)}^{2} - \frac{\alpha_{1}}{4} \norm{\mathbf{\hat{u}} - \mathbf{\hat{v}}}_{L^{2}(\mathcal{M}_{t} \setminus \Sigma)}^{2}
\end{aligned}
\end{equation*}
and we obtain the inequality
\begin{equation*}
	\frac{1}{4}\norm{\nabla_{\mathcal{M}} \hat{f} \cdot (\mathbf{\hat{u}} - \mathbf{\hat{v}})}_{L^{2}(\mathcal{M}_{t})}^{2} + \frac{\alpha_{0}}{4} \abs{\mathbf{\hat{u}} - \mathbf{\hat{v}}}_{H^{1}(\Sigma)}^{2} + \frac{\alpha_{1}}{4} \norm{\mathbf{\hat{u}} - \mathbf{\hat{v}}}_{L^{2}(\mathcal{M}_{t} \setminus \Sigma)}^{2} \le 0.
\end{equation*}
From the non-negativity of norms and the last term on the left-hand side it follows that $\mathbf{\hat{u}} = \mathbf{\hat{v}}$ on $\mathcal{M}_{t} \setminus \Sigma$.
From the second term we obtain $\nabla \mathbf{\hat{u}} = \nabla \mathbf{\hat{v}}$ on $\Sigma$.
Thus, $\mathbf{\hat{u}} - \mathbf{\hat{v}}$ is constant on $\Sigma$.
Finally, combining the first term with \eqref{eq:schnoerrineq} yields
\begin{equation*}
	\norm{\mathbf{\hat{u}} - \mathbf{\hat{v}}}_{L^{2}(\Sigma)}^{2} \lesssim \norm{\nabla_{\mathcal{M}} \hat{f} \cdot (\mathbf{\hat{u}} - \mathbf{\hat{v}})}_{L^{2}(\Sigma)}^{2},
\end{equation*}
which implies that $\mathbf{\hat{u}} - \mathbf{\hat{v}} = 0$ on $\Sigma$ and the uniqueness follows.
\end{proof}

\section{Wellposedness of Continuity Equation}

Let $t \in I$ and let $\Sigma \subseteq \mathcal{M}_{t}$.
We define the space
\begin{equation*}
	Y \coloneqq H^{1}(\Sigma) \times H^{\mathrm{div}}(\mathcal{M}_{t} \setminus \Sigma)	
\end{equation*}
with respect to the norm
\begin{equation*}
	\norm{\mathbf{\hat{u}}}_{X}^{2} \coloneqq \norm{\mathbf{\hat{u}}}_{H^{1}(\Sigma)}^{2} + \norm{\mathbf{\hat{u}}}_{H^{\mathrm{div}}(\mathcal{M}_{t} \setminus \Sigma)}^{2}.
\label{eq:normy}
\end{equation*}
Again, the norms are taken with regard to the projections $\mathbf{\hat{u}}|_{\Sigma}$ and $\mathbf{\hat{u}}|_{\mathcal{M}_{t} \setminus \Sigma}$.

We seek a minimiser to the energy $\mathcal{F}: Y \to [0, +\infty]$,
\begin{equation}
	\mathcal{F}(\mathbf{\hat{u}}) \coloneqq \norm{d_{t}^{\mathbf{\hat{N}}} \hat{f} + \nabla_{\mathcal{M}} \cdot (\hat{f} \mathbf{\hat{u}}) - \hat{f} K V}_{L^{2}(\mathcal{M}_{t})}^{2} + \mathcal{R}(\mathbf{\hat{u}}) + \mathcal{S}(\mathbf{\hat{u}}),
\label{eq:cmfunctional}
\end{equation}
where $\mathcal{R}(\mathbf{\hat{u}})$ is defined in \eqref{eq:regfunctional} and
\begin{equation}
	\mathcal{S}(\mathbf{\hat{u}}) \coloneqq \alpha_{2} \int_{\mathcal{M}_{t}} (1 - s) \bigl( \nabla_{\mathcal{M}} \cdot \mathbf{\hat{u}} \bigr)^{2} \; d\mathcal{M}_{t}.
\label{eq:regfunctional2}
\end{equation}
Here, $\alpha_{2} > 0$ is a regularisation parameter.
The reason for this additional regularisation term in contrast to \eqref{eq:offunctional} is to control oscillations in the velocity field, which may arise from the data term in the presence of noise.
% suppress spurious oscillations

\begin{theorem}
Let $\hat{f} \in W^{1, \infty}(\mathcal{M}_{t})$, $d_{t}^{\mathbf{\hat{N}}} \hat{f} \in L^{2}(\mathcal{M}_{t})$, and let $\hat{f} K V \in L^{2}(\mathcal{M}_{t})$.
Moreover, let $\hat{f}$, $\y$, and $\Sigma$ satisfy assumptions of Lemmata~\ref{lem:poincarewirtinger} and \ref{lem:schnoerrineq}.
Then, there exists a unique minimiser of $\mathcal{F}$ in the space $Y$.
\end{theorem}
\begin{proof}
The proof is along the lines of the proof of Thm.~\ref{thm:ofwellposedness}.
Assume that $\Sigma \subset \mathcal{M}_{t}$.
From non-negativity of $\mathcal{F}$, the assumptions on $\hat{f}$ and $\hat{f} K V$ we find that $\mathcal{F}$ is proper.
By the same arguments as before we obtain
\begin{align*}
	\norm{\mathbf{\hat{u}}}_{Y}^{2} & = \norm{\mathbf{\hat{u}}}_{L^{2}(\Sigma)}^{2} + \abs{\mathbf{\hat{u}}}_{H^{1}(\Sigma)}^{2} + \norm{\mathbf{\hat{u}}}_{H^{\mathrm{div}}(\mathcal{M}_{t} \setminus \Sigma)}^{2} \\
	& \lesssim \norm{(\mathbf{\hat{u}})_{\Sigma}}_{L^{2}(\Sigma)}^{2} + \norm{\mathbf{\hat{u}} - (\mathbf{\hat{u}})_{\Sigma}}_{L^{2}(\Sigma)}^{2} + \abs{\mathbf{\hat{u}}}_{H^{1}(\Sigma)}^{2} + \norm{\mathbf{\hat{u}}}_{H^{\mathrm{div}}(\mathcal{M}_{t} \setminus \Sigma)}^{2} \\
	& \overset{\mathclap{\eqref{eq:poincareineq}}}{\lesssim} \norm{(\mathbf{\hat{u}})_{\Sigma}}_{L^{2}(\Sigma)}^{2} + \abs{\mathbf{\hat{u}}}_{H^{1}(\Sigma)}^{2} + \norm{\mathbf{\hat{u}}}_{H^{\mathrm{div}}(\mathcal{M}_{t} \setminus \Sigma)}^{2} \\
	& \overset{\mathclap{\eqref{eq:schnoerrineq}}}{\lesssim} \norm{\nabla_{\mathcal{M}} \hat{f} \cdot (\mathbf{\hat{u}})_{\Sigma}}_{L^{2}(\Sigma)}^{2} + \abs{\mathbf{\hat{u}}}_{H^{1}(\Sigma)}^{2} + \norm{\mathbf{\hat{u}}}_{H^{\mathrm{div}}(\mathcal{M}_{t} \setminus \Sigma)}^{2} \\
	& \lesssim \norm{\nabla_{\mathcal{M}} \hat{f} \cdot \mathbf{\hat{u}}}_{L^{2}(\Sigma)}^{2} + \norm{\nabla_{\mathcal{M}} \hat{f} \cdot (\mathbf{\hat{u}} - (\mathbf{\hat{u}})_{\Sigma})}_{L^{2}(\Sigma)}^{2} + \abs{\mathbf{\hat{u}}}_{H^{1}(\Sigma)}^{2} + \norm{\mathbf{\hat{u}}}_{H^{\mathrm{div}}(\mathcal{M}_{t} \setminus \Sigma)}^{2} \\
	& \lesssim \norm{\nabla_{\mathcal{M}} \hat{f} \cdot \mathbf{\hat{u}}}_{L^{2}(\mathcal{M}_{t})}^{2} + \abs{\mathbf{\hat{u}}}_{H^{1}(\Sigma)}^{2} + \norm{\mathbf{\hat{u}}}_{H^{\mathrm{div}}(\mathcal{M}_{t} \setminus \Sigma)}^{2} \\
	& \lesssim \mathcal{F}(\mathbf{\hat{u}}) + \norm{d_{t}^{\mathbf{\hat{N}}} \hat{f}}_{L^{2}(\mathcal{M}_{t})}^{2} + \norm{\hat{f} K V}_{L^{2}(\mathcal{M}_{t})}^{2},
\end{align*}
where the last inequality follows from the application of Young's inequality to
\begin{equation*}
	\norm{\nabla_{\mathcal{M}} \cdot \mathbf{\hat{u}}}_{L^{2}(\Sigma)}^{2} \overset{\mathclap{\eqref{eq:surfdiv}}}{=} \int_{\Sigma} (\mathfrak{D}_{i} \mathfrak{u}^{i})^{2} \; d\Sigma \lesssim \int_{\Sigma} \sum_{i, k} (\mathfrak{D}_{i} \mathfrak{u}^{k})^{2} \; d\Sigma \overset{\mathclap{\eqref{eq:h1seminorm}}}{=}  \abs{\mathbf{\hat{u}}}_{H^{1}(\Sigma)}^{2}.
\end{equation*}
Thus, $\mathcal{F}$ is coercive.

Weak lower-semicontinuity of $\mathcal{F}|_{\Sigma}$ is along the lines of the proof of Thm.~\ref{thm:ofwellposedness}.
For $\mathcal{F}|_{\mathcal{M}_{t} \setminus \Sigma}$ we note that, for a sequence $\{ \mathbf{\hat{w}}_{n} \} \subset H^{\mathrm{div}}(\mathcal{M}_{t} \setminus \Sigma)$ converging  to $\mathbf{\hat{w}}_{0}$ in the weak topology of $H^{\mathrm{div}}(\mathcal{M}_{t} \setminus \Sigma)$, we have that both $\mathbf{\hat{w}}_{n} \rightharpoonup \mathbf{\hat{w}}_{0}$ and $\nabla \cdot \mathbf{\hat{w}}_{n} \rightharpoonup \nabla \cdot \mathbf{\hat{w}}_{0}$ in $L^{2}(\mathcal{M}_{t} \setminus \Sigma)$.
By application of \cite[Thm.~3.20]{Dac08} and the weak lower-semicontinuity of norms, the weak lower-semicontinuity of $\mathcal{F}$ follows and allows us to conclude the existence of a minimiser.

Uniqueness is analogous to the proof of Thm.~\ref{thm:ofwellposedness}.
By adjusting the first equality to the modified data term and by adding another equality with $u = \nabla_{\mathcal{M}} \cdot \mathbf{\hat{u}}$ and $v = \nabla_{\mathcal{M}} \cdot \mathbf{\hat{v}}$ for $U = \mathcal{M}_{t} \setminus \Sigma$ we arrive at
\begin{equation*}
\begin{aligned}
	\frac{1}{4}\norm{\nabla_{\mathcal{M}} \cdot (\hat{f} \mathbf{\hat{u}} - \hat{f} \mathbf{\hat{v}})}_{L^{2}(\mathcal{M}_{t})}^{2} + \frac{\alpha_{0}}{4} \abs{\mathbf{\hat{u}} - \mathbf{\hat{v}}}_{H^{1}(\Sigma)}^{2} + \frac{\alpha_{1}}{4} \norm{\mathbf{\hat{u}} - \mathbf{\hat{v}}}_{L^{2}(\mathcal{M}_{t} \setminus \Sigma)}^{2} \\
	+ \frac{\alpha_{2}}{4} \norm{\nabla_{\mathcal{M}} \cdot (\mathbf{\hat{u}} - \mathbf{\hat{v}})}_{L^{2}(\mathcal{M}_{t} \setminus \Sigma)}^{2} \le 0.
\end{aligned}
\end{equation*}
With the same argumentation we find that $\mathbf{\hat{u}} = \mathbf{\hat{v}}$ on $\mathcal{M}_{t} \setminus \Sigma$, moreover that $\mathbf{\hat{u}} - \mathbf{\hat{v}}$ is constant on $\Sigma$, and by
\begin{equation*}
	\norm{\mathbf{\hat{u}} - \mathbf{\hat{v}}}_{L^{2}(\Sigma)}^{2} \overset{\mathclap{\eqref{eq:schnoerrineq}}}{\lesssim} \norm{\nabla_{\mathcal{M}} \hat{f} \cdot (\mathbf{\hat{u}} - \mathbf{\hat{v}})}_{L^{2}(\Sigma)}^{2} = \norm{\nabla_{\mathcal{M}} \cdot (\hat{f} \mathbf{\hat{u}} - \hat{f} \mathbf{\hat{v}})}_{L^{2}(\Sigma)}^{2} ,
\end{equation*}
that $\mathbf{\hat{u}} - \mathbf{\hat{v}} = 0$ on $\Sigma$.
Uniqueness of a minimiser follows.
\end{proof}

\section{Deferred Proofs} \label{sec:deferredproofs}

\begin{proof}[Proof of Lemma~\ref{lem:poincarewirtinger}]
Suppose to the contrary there exists no $C > 0$ such that the inequality holds.
Then, for all $n \in \N$ there exists a tangent vector field $\mathbf{\hat{w}}_{n} \in H^{1}(\Sigma)$ satisfying
\begin{equation*}
	\norm{\mathbf{\hat{w}}_{n} - (\mathbf{\hat{w}}_{n})_{\Sigma}}_{L^{2}(\Sigma)}^{2} > n \abs{\mathbf{\hat{w}}_{n}}_{H^{1}(\Sigma)}^{2}.
\end{equation*}
We rescale and define for every $n \in \N$,
\begin{equation*}
	\mathbf{\hat{v}}_{n} \coloneqq \frac{\mathbf{\hat{w}}_{n} - (\mathbf{\hat{w}}_{n})_{\Sigma}}{\norm{\mathbf{\hat{w}}_{n} - (\mathbf{\hat{w}}_{n})_{\Sigma}}_{L^{2}(\Sigma)}}
\end{equation*}
Then, $(v_{n}^{i})_{\Sigma} = 0$ and $\norm{\mathbf{\hat{v}}_{n}}_{L^{2}(\Sigma)} = 1$ and, for all $n \in \N$,
\begin{equation}
	\abs{\mathbf{\hat{v}}_{n}}_{H^{1}(\Sigma)}^{2} < \frac{1}{n}.
\label{eq:decreasingseminorm}
\end{equation}
As a consequence, all $\mathbf{\hat{v}}_{n}$ are bounded in $H^{1}(\Sigma)$.

By Kondrakov's Theorem for Riemannian manifolds~\cite[Thm.~2.34]{Aub82}, there exists a subsequence $\{\mathbf{\hat{v}}_{n_{k}}\}$ and a tangent vector field $\mathbf{\hat{v}} \in L^{2}(\Sigma)$ such that
\begin{equation*}
\mathbf{\hat{v}}_{n_{k}} \to \mathbf{\hat{v}} \text{ in $L^{2}(\Sigma)$}.
\end{equation*}
It follows that $(v^{i})_{\Sigma} = 0$ and $\norm{\mathbf{\hat{v}}}_{L^{2}(\Sigma)} = 1$.

On the other hand, from integration by parts and the divergence theorem it follows that, for all $\hat{h} \in C_{c}^{\infty}(\Sigma)$,
\begin{equation*}
\begin{aligned}
	\int_{\Sigma} \nabla_{\mathcal{M}} \hat{h} \cdot \mathbf{\hat{v}} \; d\Sigma & = \lim_{k \to \infty} \int_{\Sigma} \nabla_{\mathcal{M}} \hat{h} \cdot \mathbf{\hat{v}}_{n_{k}} \; d\Sigma \\
	& = \lim_{k \to \infty} \int_{\Sigma} \nabla_{\mathcal{M}} \cdot (\hat{h} \mathbf{\hat{v}}_{n_{k}}) \; d\Sigma - \int_{\Sigma} \hat{h} \nabla_{\mathcal{M}} \cdot \mathbf{\hat{v}}_{n_{k}} \; d\Sigma \\
	& = \lim_{k \to \infty} \int_{\partial \Sigma} \hat{h} \mathbf{\hat{v}}_{n_{k}} \cdot \boldsymbol{\hat{\nu}} \; dS - \int_{\Sigma} \hat{h} \nabla_{\mathcal{M}} \cdot \mathbf{\hat{v}}_{n_{k}} \; d\Sigma \\
	& = 0.
\end{aligned}
\end{equation*}
Here, the last identity follows from the choice of $\hat{h}$ and the fact that, by \eqref{eq:decreasingseminorm}, we have $\abs{\mathbf{\hat{v}}_{n_{k}}}_{H^{1}(\Sigma)}^{2} \to 0$ which, for a representation $\mathbf{\hat{v}}_{n_{k}} = \mathfrak{v}_{n_{k}}^{i} \mathbf{\hat{e}}_{i}$ in an orthonormal basis, implies $(\mathfrak{D}_{i}\mathfrak{v}_{n_{k}}^{j})^{2} \to 0$ a.e., cf. proof of Lemma~\ref{lem:covderiv}. In particular, it implies $\mathfrak{D}_{i}\mathfrak{v}_{n_{k}}^{i} \to 0$ a.e. which implies $\nabla_{\mathcal{M}} \cdot \mathbf{\hat{v}}_{n_{k}} \to 0$ a.e., see definition \eqref{eq:surfdiv}.

As a consequence, $\mathbf{\hat{v}} \in H^{1}(\Sigma)$ with $\nabla \mathbf{\hat{v}} = 0$ a.e.
Since $\Sigma$ is connected it follows that $\mathbf{\hat{v}}$ is covariantly constant.
But since $(v^{i})_{\Sigma} = 0$ we must have $\mathbf{\hat{v}} = 0$, which contradicts the fact that $\norm{\mathbf{\hat{v}}}_{L^{2}(\Sigma)} = 1$.
Therefore, inequality \eqref{eq:poincareineq} holds.
\end{proof}

\begin{proof}[Proof of Lemma~\ref{lem:schnoerrineq}]
We assume $\norm{\mathbf{\hat{w}}_{n}}_{L^{2}(\Sigma)} \neq 0$.
Suppose for the contrary that there is no $C > 0$ such that the inequality holds.
Then, for all $n \in \N$ there exists $\mathbf{\hat{w}}_{n} \in L^{2}(\Sigma)$ such that
\begin{equation*}
	\norm{\nabla_{\mathcal{M}} \hat{f} \cdot \mathbf{\hat{w}}_{n}}_{L^{2}(\Sigma)}^{2} < \frac{1}{n} \norm{\mathbf{\hat{w}}_{n}}_{L^{2}(\Sigma)}^{2}.
\end{equation*}
We let $\mathbf{\hat{v}}_{n} = \mathbf{\hat{w}}_{n} / \norm{\mathbf{\hat{w}}_{n}}_{L^{2}(\Sigma)}$ and obtain
\begin{equation*}
	\norm{\nabla_{\mathcal{M}} \hat{f} \cdot \mathbf{\hat{v}}_{n}}_{L^{2}(\Sigma)}^{2} < \frac{1}{n}.
\end{equation*}
But then,
\begin{align*}
	\frac{1}{n} & > \norm{\nabla_{\mathcal{M}} \hat{f} \cdot \mathbf{\hat{v}}_{n}}_{L^{2}(\Sigma)}^{2} \\
	& \overset{\mathclap{\eqref{eq:surfgradip}}}{=} \norm{\partial_{i} f v_{n}^{i}}_{L^{2}(\Sigma)}^{2} \\
	& = \norm{\partial_{1} f v_{n}^{1}}_{L^{2}(\Sigma)}^{2} + \norm{\partial_{2} f v_{n}^{2}}_{L^{2}(\Sigma)}^{2} + 2 \langle \partial_{1} f v_{n}^{1}, \partial_{2} f v_{n}^{2} \rangle_{L^{2}(\Sigma)} \\
	& \ge \norm{\partial_{1} f v_{n}^{1}}_{L^{2}(\Sigma)}^{2} + \norm{\partial_{2} f v_{n}^{2}}_{L^{2}(\Sigma)}^{2} \\
	& \qquad - 2 \norm{\partial_{1} f v_{n}^{1}}_{L^{2}(\Sigma)} \norm{\partial_{2} f v_{n}^{2}}_{L^{2}(\Sigma)}	\frac{\abs{\langle \partial_{1} f v_{n}^{1}, \partial_{2} f v_{n}^{2} \rangle_{L^{2}(\Sigma)}}}{\norm{\partial_{1} f v_{n}^{1}}_{L^{2}(\Sigma)} \norm{\partial_{2} f v_{n}^{2}}_{L^{2}(\Sigma)}} \\
	& \ge \left( \norm{\partial_{1} f v_{n}^{1}}_{L^{2}(\Sigma)}^{2} + \norm{\partial_{2} f v_{n}^{2}}_{L^{2}(\Sigma)}^{2} \right) \left( 1 - \frac{\abs{\langle \partial_{1} f v_{n}^{1}, \partial_{2} f v_{n}^{2} \rangle_{L^{2}(\Sigma)}}}{\norm{\partial_{1} f v_{n}^{1}}_{L^{2}(\Sigma)} \norm{\partial_{2} f v_{n}^{2}}_{L^{2}(\Sigma)}} \right) \\
	& = \left( (v_{n}^{1})^{2} \norm{\partial_{1} f}_{L^{2}(\Sigma)}^{2} + (v_{n}^{2})^{2} \norm{\partial_{2} f}_{L^{2}(\Sigma)}^{2} \right) \left( 1 - \frac{\abs{\langle \partial_{1} f, \partial_{2} f \rangle_{L^{2}(\Sigma)}}}{\norm{\partial_{1} f}_{L^{2}(\Sigma)} \norm{\partial_{2} f}_{L^{2}(\Sigma)}} \right)
\end{align*}
together with \eqref{eq:linindep} implies that $v_{n}^{1}, v_{n}^{2} \to 0$ as $n \to \infty$, contradicting the assumption.
Here, the second inequality arises from application of Young's inequality.
\end{proof}
